# Supplementary material for: AITP: Traffic Accident Responsibility Allocation via Multimodal Large Language Models
Source: arXiv:2604.20878 source file (2026-04-11)
Supplement: Supplementary file 1 [file 12_appendix.tex]

\section{Appendix Section}
\label{sec:appendix_section}
Supplementary material goes here.
